# Supplementary material for: GenAI-Net: A Generative AI Framework for Automated Biomolecular Network Design
Source: arXiv:2601.17582 ancillary file (2026-02-27)

# GenAI-Net: A Generative AI Framework for Automated Biomolecular Network Design

*Supplementary Material: Discovered networks structure and parameters*

Maurice Filo, Nicolò Rossi, Zhou Fang, Mustafa Khammash

## 1 Task: Dose-Response

In this task, the networks are designed so that the steady-state concentration of the output species follows a specific functional form relative to the input  $u_1$ .

### 1.1 Hill-function Mapping (3 Species, 5 Reactions)

The following networks approximate a sigmoidal Hill-type response, characterized by sensitivity to a threshold concentration of the input.

#### I/O CRN 1

Loss: 0.01622

Inputs:  $\{u_1\}$     Species:  $\{X_1, X_2, X_3\}$     Output:  $X_3$

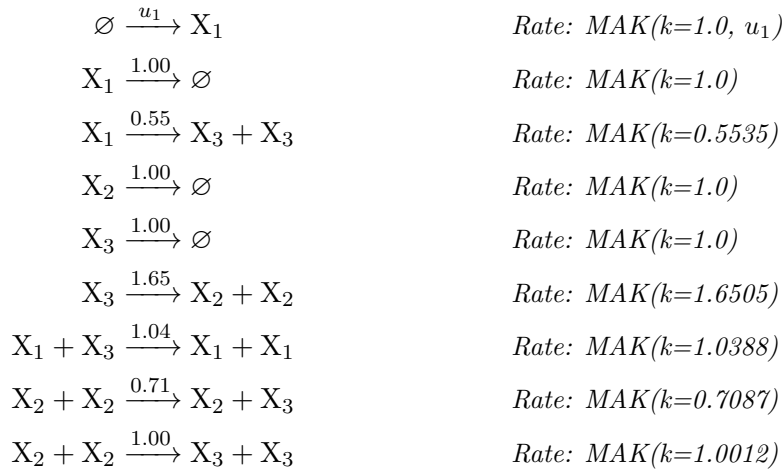

#### I/O CRN 4

Loss: 0.01912

Inputs:  $\{u_1\}$     Species:  $\{X_1, X_2, X_3\}$     Output:  $X_3$

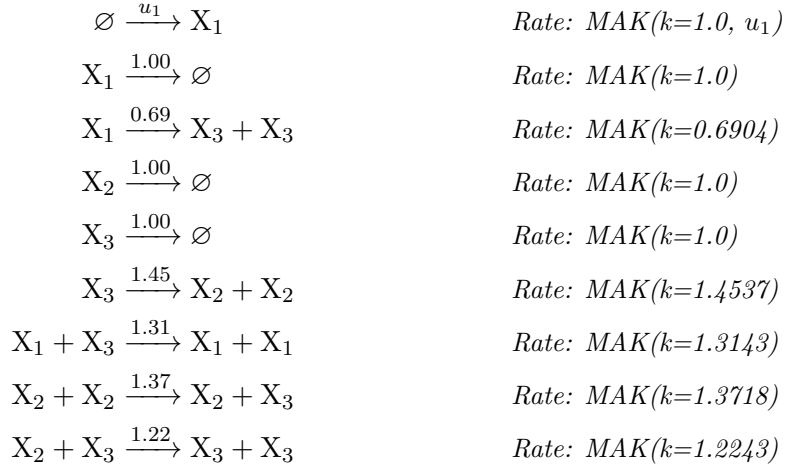

### I/O CRN 8

Loss: 0.02026

Inputs:  $\{u_1\}$     Species:  $\{X_1, X_2, X_3\}$     Output:  $X_3$

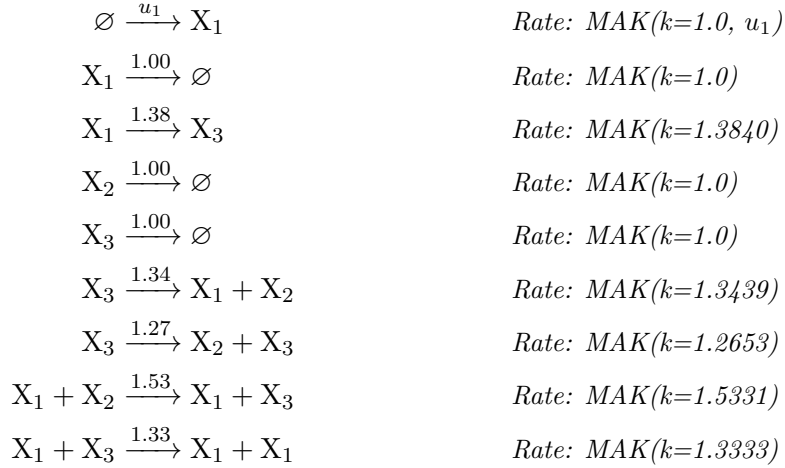

## 1.2 Ultra-Sensitive Mapping (3 Species, 5 Reactions)

This subsection details the networks optimized for Ultra-Sensitive responses, characterized by a very steep "switch-like" transition in output concentration over a narrow range of input values. These are typically achieved through mechanisms like zero-order ultrasensitivity or molecular titration.

### I/O CRN 1

Loss: 0.01380

Inputs:  $\{u_1\}$     Species:  $\{X_1, X_2, X_3\}$     Output:  $X_3$

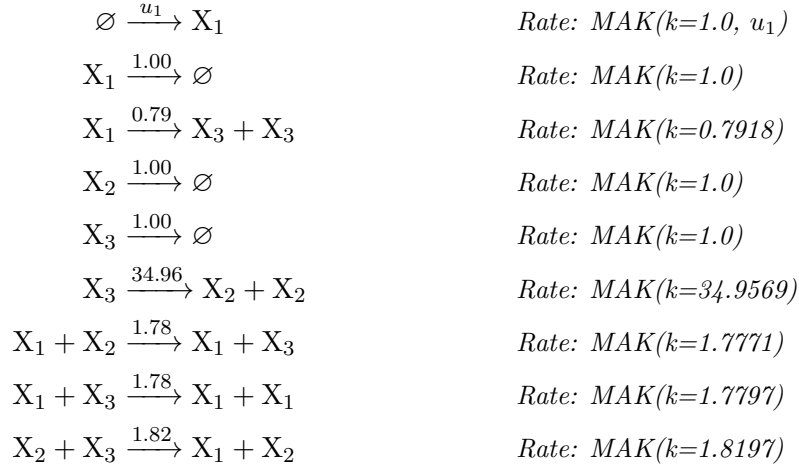

### I/O CRN 20

Loss: 0.02082

Inputs:  $\{u_1\}$     Species:  $\{X_1, X_2, X_3\}$     Output:  $X_3$

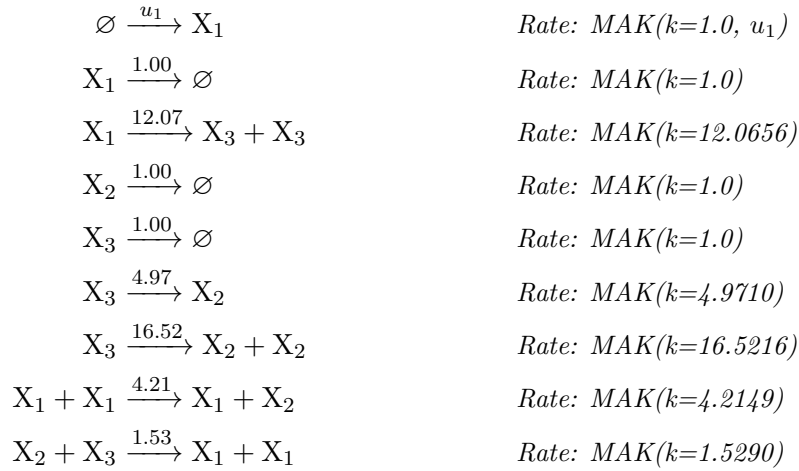

### 1.3 Biphasic Mapping (3 Species, 5 Reactions)

This subsection presents networks that exhibit a Biphasic (or bell-shaped) response. In these systems, the output concentration initially increases with the input stimulus  $u_1$ , but subsequently decreases as the input concentration continues to rise.

#### I/O CRN 1

Loss: 0.05380

Inputs:  $\{u_1\}$     Species:  $\{X_1, X_2, X_3\}$     Output:  $X_3$

|                                          |                                                        |
|------------------------------------------|--------------------------------------------------------|
| $\emptyset \xrightarrow{u_1} X_1$        | <i>Rate: MAK(<math>k=1.0</math>, <math>u_1</math>)</i> |
| $X_1 \xrightarrow{1.00} \emptyset$       | <i>Rate: MAK(<math>k=1.0</math>)</i>                   |
| $X_2 \xrightarrow{1.00} \emptyset$       | <i>Rate: MAK(<math>k=1.0</math>)</i>                   |
| $X_2 \xrightarrow{0.74} X_1 + X_2$       | <i>Rate: MAK(<math>k=0.7361</math>)</i>                |
| $X_3 \xrightarrow{1.00} \emptyset$       | <i>Rate: MAK(<math>k=1.0</math>)</i>                   |
| $X_3 \xrightarrow{0.57} X_1 + X_2$       | <i>Rate: MAK(<math>k=0.5742</math>)</i>                |
| $X_1 + X_1 \xrightarrow{0.44} X_3 + X_3$ | <i>Rate: MAK(<math>k=0.4442</math>)</i>                |
| $X_1 + X_2 \xrightarrow{0.39} X_2 + X_2$ | <i>Rate: MAK(<math>k=0.3872</math>)</i>                |
| $X_2 + X_3 \xrightarrow{0.70} X_1 + X_2$ | <i>Rate: MAK(<math>k=0.6972</math>)</i>                |

---

## I/O CRN 12

**Loss:** 0.06556

**Inputs:**  $\{u_1\}$    **Species:**  $\{X_1, X_2, X_3\}$    **Output:**  $X_3$

|                                          |                                                        |
|------------------------------------------|--------------------------------------------------------|
| $\emptyset \xrightarrow{u_1} X_1$        | <i>Rate: MAK(<math>k=1.0</math>, <math>u_1</math>)</i> |
| $X_1 \xrightarrow{1.00} \emptyset$       | <i>Rate: MAK(<math>k=1.0</math>)</i>                   |
| $X_2 \xrightarrow{1.00} \emptyset$       | <i>Rate: MAK(<math>k=1.0</math>)</i>                   |
| $X_3 \xrightarrow{1.00} \emptyset$       | <i>Rate: MAK(<math>k=1.0</math>)</i>                   |
| $X_1 + X_1 \xrightarrow{0.57} X_3 + X_3$ | <i>Rate: MAK(<math>k=0.5680</math>)</i>                |
| $X_1 + X_2 \xrightarrow{0.79} X_2 + X_2$ | <i>Rate: MAK(<math>k=0.7884</math>)</i>                |
| $X_2 + X_3 \xrightarrow{0.37} X_1 + X_1$ | <i>Rate: MAK(<math>k=0.3690</math>)</i>                |
| $X_2 + X_3 \xrightarrow{0.52} X_1 + X_2$ | <i>Rate: MAK(<math>k=0.5194</math>)</i>                |
| $X_3 + X_3 \xrightarrow{0.29} X_2 + X_3$ | <i>Rate: MAK(<math>k=0.2924</math>)</i>                |

## 2 Task: Robust Perfect Adaptation

This section details the In-Silico Optimized Chemical Reaction Networks (I/O CRNs) discovered for the Robust Perfect Adaptation task. Reaction rates (rounded to 2 decimal places) are displayed above the arrows, with full parameter details provided on the right.

### 2.1 Configuration: 3 Species, 5 Reactions

#### I/O CRN 1

**Loss:** 0.00292

**Inputs:**  $\{u_1, u_2\}$    **Species:**  $\{X_1, Z_1, Z_2\}$    **Output:**  $X_1$

|                                          |                                           |
|------------------------------------------|-------------------------------------------|
| $\emptyset \xrightarrow{u_1} Z_1$        | <i>Rate: MAK(<math>k=1.0, u_1</math>)</i> |
| $\emptyset \xrightarrow{0.95} X_1 + X_1$ | <i>Rate: MAK(<math>k=0.9523</math>)</i>   |
| $X_1 \xrightarrow{u_2} \emptyset$        | <i>Rate: MAK(<math>k=1.0, u_2</math>)</i> |
| $X_1 \xrightarrow{1.00} Z_2$             | <i>Rate: MAK(<math>k=1.0007</math>)</i>   |
| $Z_1 \xrightarrow{3.11} X_1 + Z_1$       | <i>Rate: MAK(<math>k=3.1131</math>)</i>   |
| $X_1 + Z_2 \xrightarrow{2.85} Z_2$       | <i>Rate: MAK(<math>k=2.8472</math>)</i>   |
| $Z_1 + Z_2 \xrightarrow{1.03} \emptyset$ | <i>Rate: MAK(<math>k=1.0346</math>)</i>   |

---

### I/O CRN 19

**Loss:** 0.00519

**Inputs:**  $\{u_1, u_2\}$    **Species:**  $\{X_1, Z_1, Z_2\}$    **Output:**  $X_1$

|                                          |                                           |
|------------------------------------------|-------------------------------------------|
| $\emptyset \xrightarrow{u_1} Z_1$        | <i>Rate: MAK(<math>k=1.0, u_1</math>)</i> |
| $X_1 \xrightarrow{u_2} \emptyset$        | <i>Rate: MAK(<math>k=1.0, u_2</math>)</i> |
| $X_1 \xrightarrow{1.00} Z_2$             | <i>Rate: MAK(<math>k=1.0007</math>)</i>   |
| $Z_1 \xrightarrow{1.62} X_1 + Z_1$       | <i>Rate: MAK(<math>k=1.6172</math>)</i>   |
| $X_1 + X_1 \xrightarrow{1.01} \emptyset$ | <i>Rate: MAK(<math>k=1.0056</math>)</i>   |
| $X_1 + Z_2 \xrightarrow{1.02} Z_2$       | <i>Rate: MAK(<math>k=1.0227</math>)</i>   |
| $Z_1 + Z_2 \xrightarrow{1.68} X_1 + X_1$ | <i>Rate: MAK(<math>k=1.6823</math>)</i>   |

---

### I/O CRN 28

**Loss:** 0.00584

**Inputs:**  $\{u_1, u_2\}$    **Species:**  $\{X_1, Z_1, Z_2\}$    **Output:**  $X_1$

|                                          |                                           |
|------------------------------------------|-------------------------------------------|
| $\emptyset \xrightarrow{u_1} Z_1$        | <i>Rate: MAK(<math>k=1.0, u_1</math>)</i> |
| $X_1 \xrightarrow{u_2} \emptyset$        | <i>Rate: MAK(<math>k=1.0, u_2</math>)</i> |
| $X_1 \xrightarrow{1.00} Z_2$             | <i>Rate: MAK(<math>k=1.0007</math>)</i>   |
| $X_1 \xrightarrow{1.24} X_1 + X_1$       | <i>Rate: MAK(<math>k=1.2353</math>)</i>   |
| $Z_1 \xrightarrow{3.14} X_1 + Z_1$       | <i>Rate: MAK(<math>k=3.1393</math>)</i>   |
| $X_1 + X_1 \xrightarrow{1.01} Z_1 + Z_2$ | <i>Rate: MAK(<math>k=1.0059</math>)</i>   |
| $Z_1 + Z_2 \xrightarrow{1.40} \emptyset$ | <i>Rate: MAK(<math>k=1.4007</math>)</i>   |

## 2.2 Configuration: 6 Species, 8 Reactions

### I/O CRN 1

Loss: 0.00480

Inputs:  $\{u_1, u_2, u_3\}$     Species:  $\{X_1, X_2, Z_1, Z_2, Z_3, Z_4\}$     Output:  $X_2$

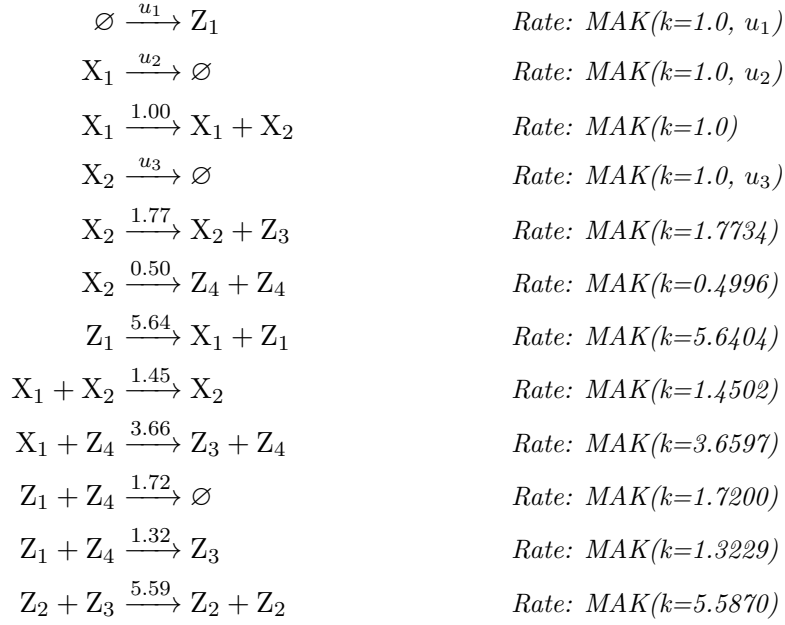

### I/O CRN 14

Loss: 0.00567

Inputs:  $\{u_1, u_2, u_3\}$     Species:  $\{X_1, X_2, Z_1, Z_3, Z_4\}$     Output:  $X_2$

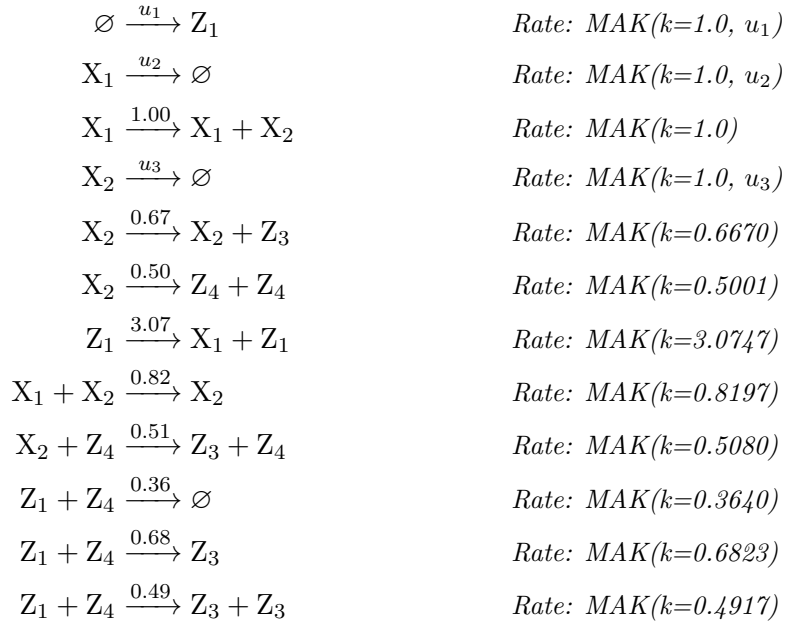

## I/O CRN 27

**Loss:** 0.00611

**Inputs:**  $\{u_1, u_2, u_3\}$     **Species:**  $\{X_1, X_2, Z_1, Z_2, Z_3, Z_4\}$     **Output:**  $X_2$

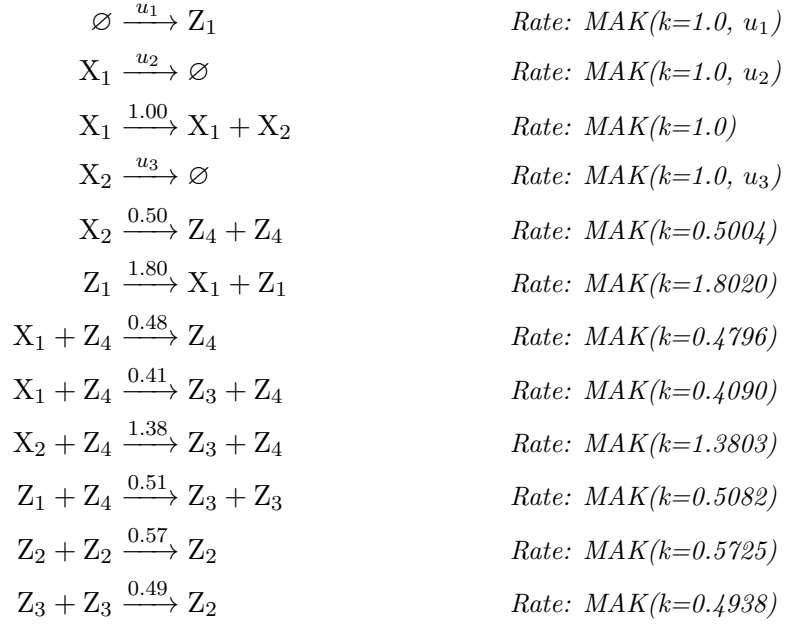

## 2.3 Configuration: 2 Species, 4 Reactions

### I/O CRN 2

Loss: 0.01230

Inputs:  $\{u_1, u_2\}$     Species:  $\{X, Z\}$     Output:  $X$

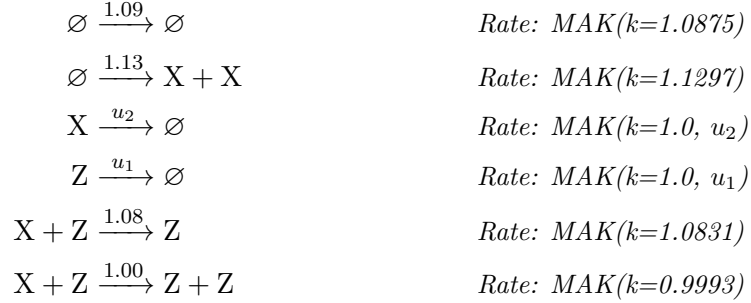

### I/O CRN 4

Loss: 0.01494

Inputs:  $\{u_1, u_2\}$     Species:  $\{X, Z\}$     Output:  $X$

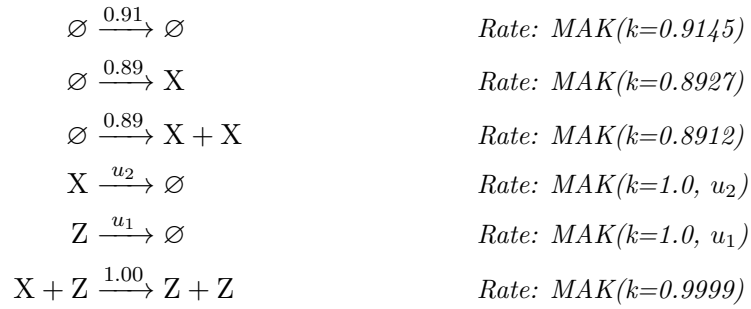

### I/O CRN 9

Loss: 0.02902

Inputs:  $\{u_1, u_2\}$     Species:  $\{X, Z\}$     Output:  $X$

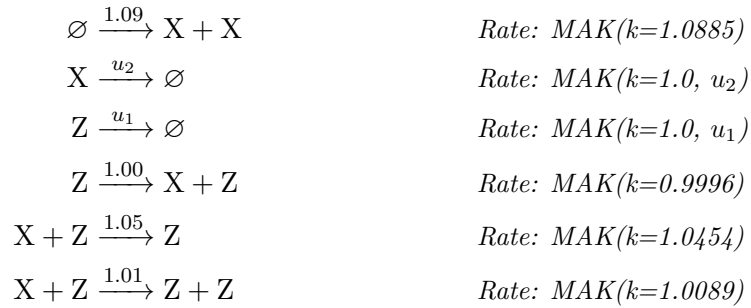

## 2.4 Configuration: 2 Species, 6 Reactions

### I/O CRN 1

Loss: 0.00059

Inputs:  $\{u_1\}$     Species:  $\{X_1, X_2\}$     Output:  $\{X_1, X_2\}$

|                                           |                                           |
|-------------------------------------------|-------------------------------------------|
| $\emptyset \xrightarrow{2.15} \emptyset$  | <i>Rate: MAK(<math>k=2.1519</math>)</i>   |
| $X_1 \xrightarrow{u_1} \emptyset$         | <i>Rate: MAK(<math>k=1.0, u_1</math>)</i> |
| $X_1 \xrightarrow{5.10} X_1 + X_1$        | <i>Rate: MAK(<math>k=5.1015</math>)</i>   |
| $X_2 \xrightarrow{1.00} \emptyset$        | <i>Rate: MAK(<math>k=1.0</math>)</i>      |
| $X_2 \xrightarrow{5.61} X_2 + X_2$        | <i>Rate: MAK(<math>k=5.6112</math>)</i>   |
| $X_1 + X_1 \xrightarrow{2.05} \emptyset$  | <i>Rate: MAK(<math>k=2.0498</math>)</i>   |
| $X_1 + X_2 \xrightarrow{15.79} \emptyset$ | <i>Rate: MAK(<math>k=15.7926</math>)</i>  |
| $X_2 + X_2 \xrightarrow{2.30} \emptyset$  | <i>Rate: MAK(<math>k=2.3049</math>)</i>   |

---

### I/O CRN 11

**Loss:** 0.00193

**Inputs:**  $\{u_1\}$    **Species:**  $\{X_1, X_2\}$    **Output:**  $\{X_1, X_2\}$

|                                          |                                           |
|------------------------------------------|-------------------------------------------|
| $\emptyset \xrightarrow{1.57} \emptyset$ | <i>Rate: MAK(<math>k=1.5695</math>)</i>   |
| $X_1 \xrightarrow{u_1} \emptyset$        | <i>Rate: MAK(<math>k=1.0, u_1</math>)</i> |
| $X_1 \xrightarrow{2.56} X_1 + X_1$       | <i>Rate: MAK(<math>k=2.5650</math>)</i>   |
| $X_2 \xrightarrow{1.00} \emptyset$       | <i>Rate: MAK(<math>k=1.0</math>)</i>      |
| $X_2 \xrightarrow{2.67} X_2 + X_2$       | <i>Rate: MAK(<math>k=2.6720</math>)</i>   |
| $X_1 + X_1 \xrightarrow{1.56} X_1$       | <i>Rate: MAK(<math>k=1.5628</math>)</i>   |
| $X_1 + X_2 \xrightarrow{4.01} \emptyset$ | <i>Rate: MAK(<math>k=4.0056</math>)</i>   |
| $X_2 + X_2 \xrightarrow{1.67} X_2$       | <i>Rate: MAK(<math>k=1.6697</math>)</i>   |

---

### I/O CRN 14

**Loss:** 0.00197

**Inputs:**  $\{u_1\}$    **Species:**  $\{X_1, X_2\}$    **Output:**  $\{X_1, X_2\}$

|                                           |                                           |
|-------------------------------------------|-------------------------------------------|
| $X_1 \xrightarrow{u_1} \emptyset$         | <i>Rate: MAK(<math>k=1.0, u_1</math>)</i> |
| $X_1 \xrightarrow{3.73} X_1 + X_1$        | <i>Rate: MAK(<math>k=3.7344</math>)</i>   |
| $X_2 \xrightarrow{1.00} \emptyset$        | <i>Rate: MAK(<math>k=1.0</math>)</i>      |
| $X_2 \xrightarrow{4.34} X_2 + X_2$        | <i>Rate: MAK(<math>k=4.3372</math>)</i>   |
| $X_1 + X_1 \xrightarrow{1.37} \emptyset$  | <i>Rate: MAK(<math>k=1.3690</math>)</i>   |
| $X_1 + X_2 \xrightarrow{13.15} \emptyset$ | <i>Rate: MAK(<math>k=13.1543</math>)</i>  |
| $X_1 + X_2 \xrightarrow{1.54} X_1$        | <i>Rate: MAK(<math>k=1.5375</math>)</i>   |
| $X_2 + X_2 \xrightarrow{1.66} \emptyset$  | <i>Rate: MAK(<math>k=1.6614</math>)</i>   |

### 3 Task: Robust Perfect Adaptation with CV Reduction

This section presents I/O CRNs optimized with stochastic simulations. These networks are designed to achieve Robust Perfect Adaptation of the mean output  $X_1$  while suppressing stochastic fluctuations (reducing the Coefficient of Variation).

#### 3.1 Configuration: 4 Species, 8 Reactions

##### I/O CRN 1

Loss: 0.20004

Inputs:  $\{u_1, u_2\}$     Species:  $\{X_1, Z_1, Z_2, Z_3\}$     Output:  $X_1$

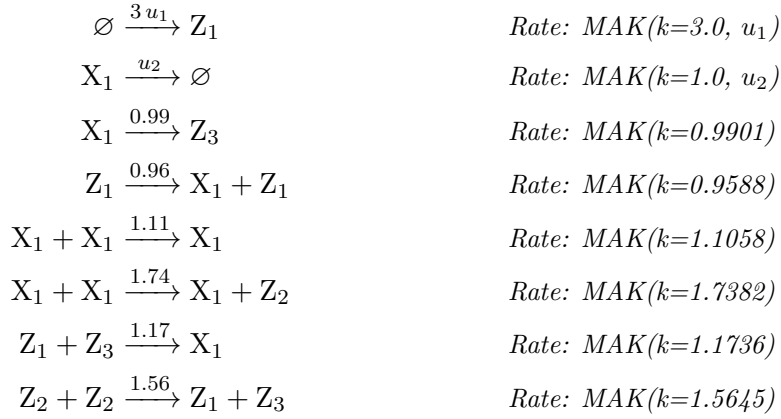

##### I/O CRN 31

Loss: 0.20772

Inputs:  $\{u_1, u_2\}$     Species:  $\{X_1, Z_1, Z_2, Z_3\}$     Output:  $X_1$

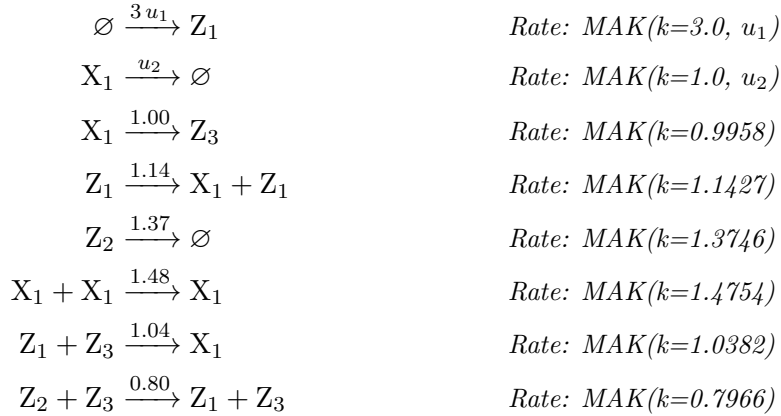

##### I/O CRN 34

Loss: 0.20897

Inputs:  $\{u_1, u_2\}$     Species:  $\{X_1, Z_1, Z_2, Z_3\}$     Output:  $X_1$

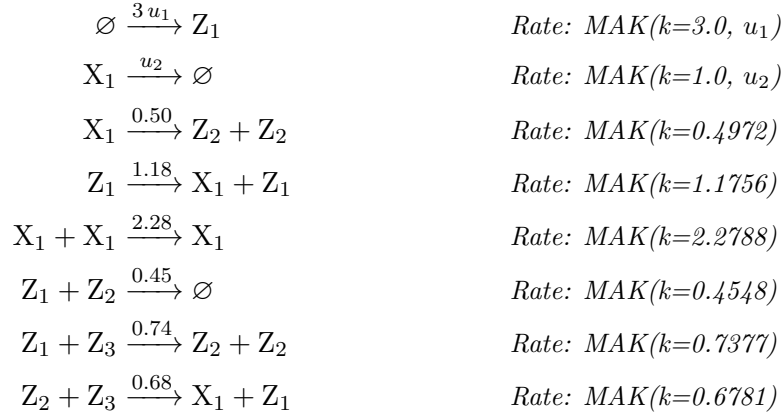

## 4 Task: Classifiers

This section describes CRNs optimized to perform classification operations across initial conditions. The output concentration of species  $X_1$  and  $X_2$  represent the classes.

### 4.1 Configuration: 2 Species, 6 Reactions

#### I/O CRN 1

**Loss:** 0.00059

**Inputs:**  $\{u_1\}$    **Species:**  $\{X_1, X_2\}$    **Output:**  $\{X_1, X_2\}$

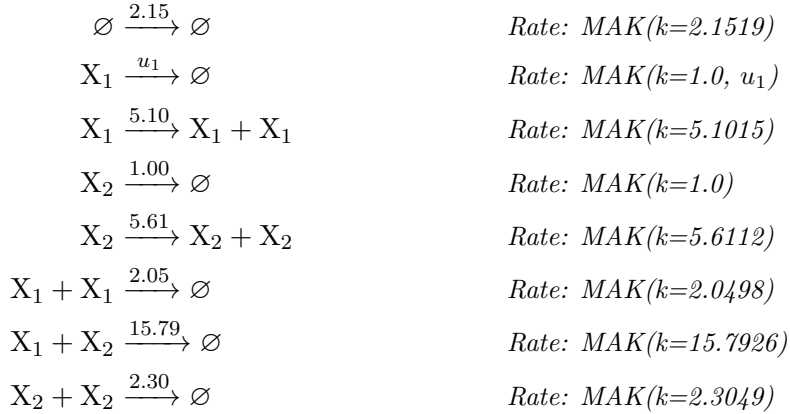


---

#### I/O CRN 11

**Loss:** 0.00193

**Inputs:**  $\{u_1\}$    **Species:**  $\{X_1, X_2\}$    **Output:**  $\{X_1, X_2\}$

|                                          |                                           |
|------------------------------------------|-------------------------------------------|
| $\emptyset \xrightarrow{1.57} \emptyset$ | <i>Rate: MAK(k=1.5695)</i>                |
| $X_1 \xrightarrow{u_1} \emptyset$        | <i>Rate: MAK(k=1.0, <math>u_1</math>)</i> |
| $X_1 \xrightarrow{2.56} X_1 + X_1$       | <i>Rate: MAK(k=2.5650)</i>                |
| $X_2 \xrightarrow{1.00} \emptyset$       | <i>Rate: MAK(k=1.0)</i>                   |
| $X_2 \xrightarrow{2.67} X_2 + X_2$       | <i>Rate: MAK(k=2.6720)</i>                |
| $X_1 + X_1 \xrightarrow{1.56} X_1$       | <i>Rate: MAK(k=1.5628)</i>                |
| $X_1 + X_2 \xrightarrow{4.01} \emptyset$ | <i>Rate: MAK(k=4.0056)</i>                |
| $X_2 + X_2 \xrightarrow{1.67} X_2$       | <i>Rate: MAK(k=1.6697)</i>                |

---

### I/O CRN 14

**Loss:** 0.00197

**Inputs:**  $\{u_1\}$    **Species:**  $\{X_1, X_2\}$    **Output:**  $\{X_1, X_2\}$

|                                           |                                           |
|-------------------------------------------|-------------------------------------------|
| $X_1 \xrightarrow{u_1} \emptyset$         | <i>Rate: MAK(k=1.0, <math>u_1</math>)</i> |
| $X_1 \xrightarrow{3.73} X_1 + X_1$        | <i>Rate: MAK(k=3.7344)</i>                |
| $X_2 \xrightarrow{1.00} \emptyset$        | <i>Rate: MAK(k=1.0)</i>                   |
| $X_2 \xrightarrow{4.34} X_2 + X_2$        | <i>Rate: MAK(k=4.3372)</i>                |
| $X_1 + X_1 \xrightarrow{1.37} \emptyset$  | <i>Rate: MAK(k=1.3690)</i>                |
| $X_1 + X_2 \xrightarrow{13.15} \emptyset$ | <i>Rate: MAK(k=13.1543)</i>               |
| $X_1 + X_2 \xrightarrow{1.54} X_1$        | <i>Rate: MAK(k=1.5375)</i>                |
| $X_2 + X_2 \xrightarrow{1.66} \emptyset$  | <i>Rate: MAK(k=1.6614)</i>                |

## 5 Task: Logic Circuits

This section describes CRNs optimized to perform logic operations across four chemical inputs. The output concentration of species OUT represents the boolean result of the computation.

### 5.1 Configuration: 5 Species, 5 Reactions

#### I/O CRN 1

Loss: 0.02127

Inputs:  $\{u_1, u_2, u_3, u_4\}$  Species:  $\{\text{OUT}, X_1, X_2, X_3, X_4\}$  Output: OUT

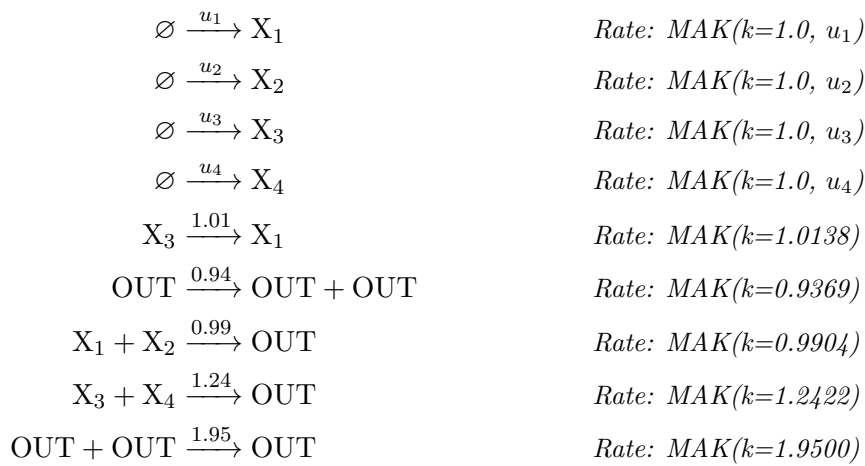

#### I/O CRN 6

Loss: 0.02274

Inputs:  $\{u_1, u_2, u_3, u_4\}$  Species:  $\{\text{OUT}, X_1, X_2, X_3, X_4\}$

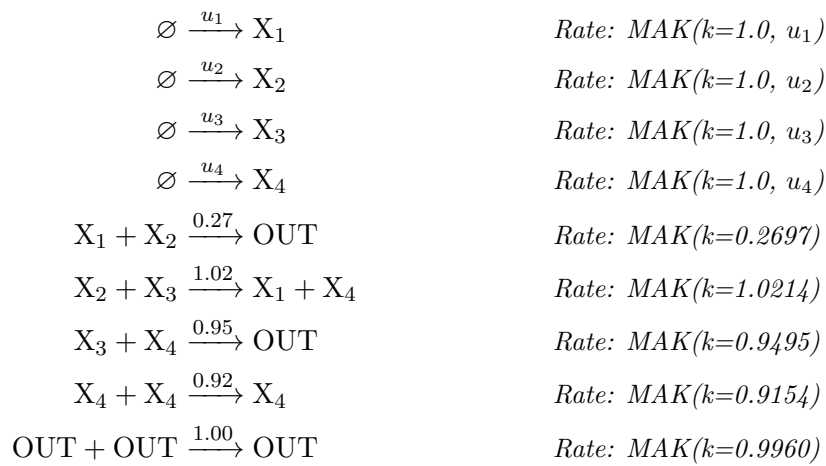

#### I/O CRN 26

Loss: 0.02468

Inputs:  $\{u_1, u_2, u_3, u_4\}$  Species:  $\{\text{OUT}, X_1, X_2, X_3, X_4\}$

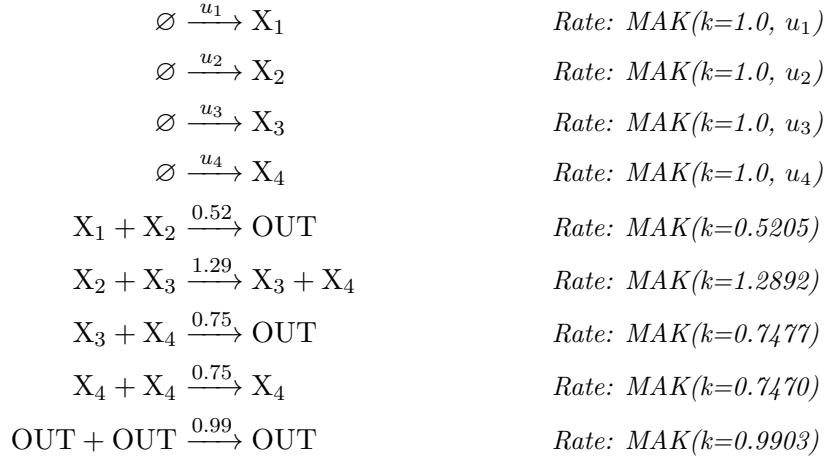

## 5.2 Configuration: 5 Species, 6 Reactions

### I/O CRN 1

**Loss:** 0.00581

**Inputs:**  $\{u_1, u_2, u_3, u_4\}$     **Species:**  $\{\text{OUT}, X_1, X_2, X_3, X_4\}$

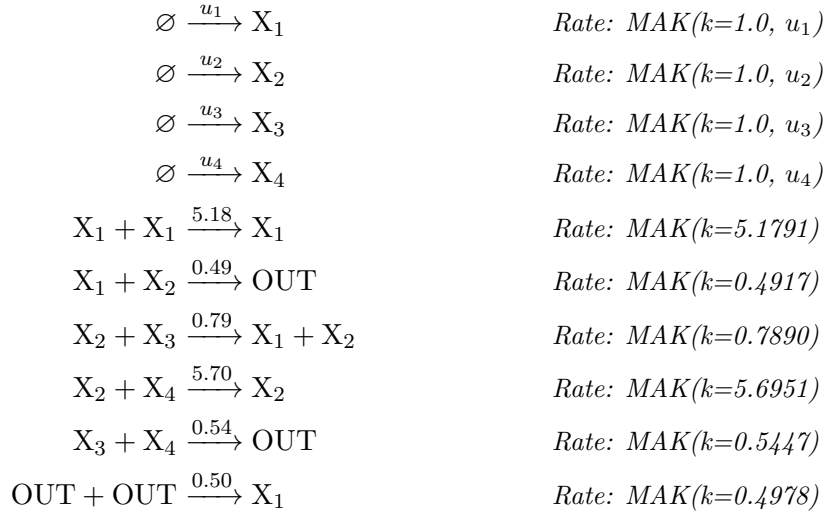


---

### I/O CRN 3

**Loss:** 0.00793

**Inputs:**  $\{u_1, u_2, u_3, u_4\}$     **Species:**  $\{\text{OUT}, X_1, X_2, X_3, X_4\}$

|                                                         |                                                        |
|---------------------------------------------------------|--------------------------------------------------------|
| $\emptyset \xrightarrow{u_1} X_1$                       | <i>Rate: MAK(<math>k=1.0</math>, <math>u_1</math>)</i> |
| $\emptyset \xrightarrow{u_2} X_2$                       | <i>Rate: MAK(<math>k=1.0</math>, <math>u_2</math>)</i> |
| $\emptyset \xrightarrow{u_3} X_3$                       | <i>Rate: MAK(<math>k=1.0</math>, <math>u_3</math>)</i> |
| $\emptyset \xrightarrow{u_4} X_4$                       | <i>Rate: MAK(<math>k=1.0</math>, <math>u_4</math>)</i> |
| $X_1 + X_2 \xrightarrow{0.10} \text{OUT}$               | <i>Rate: MAK(<math>k=0.1032</math>)</i>                |
| $X_1 + X_3 \xrightarrow{0.74} X_3$                      | <i>Rate: MAK(<math>k=0.7439</math>)</i>                |
| $X_2 + X_3 \xrightarrow{3.66} X_3 + X_4$                | <i>Rate: MAK(<math>k=3.6633</math>)</i>                |
| $X_3 + X_4 \xrightarrow{1.04} \text{OUT}$               | <i>Rate: MAK(<math>k=1.0372</math>)</i>                |
| $X_4 + X_4 \xrightarrow{0.74} \emptyset$                | <i>Rate: MAK(<math>k=0.7436</math>)</i>                |
| $\text{OUT} + \text{OUT} \xrightarrow{0.98} \text{OUT}$ | <i>Rate: MAK(<math>k=0.9819</math>)</i>                |

---

### I/O CRN 8

**Loss:** 0.01125

**Inputs:**  $\{u_1, u_2, u_3, u_4\}$     **Species:**  $\{\text{OUT}, X_1, X_2, X_3, X_4\}$

|                                                        |                                                        |
|--------------------------------------------------------|--------------------------------------------------------|
| $\emptyset \xrightarrow{u_1} X_1$                      | <i>Rate: MAK(<math>k=1.0</math>, <math>u_1</math>)</i> |
| $\emptyset \xrightarrow{u_2} X_2$                      | <i>Rate: MAK(<math>k=1.0</math>, <math>u_2</math>)</i> |
| $\emptyset \xrightarrow{u_3} X_3$                      | <i>Rate: MAK(<math>k=1.0</math>, <math>u_3</math>)</i> |
| $\emptyset \xrightarrow{u_4} X_4$                      | <i>Rate: MAK(<math>k=1.0</math>, <math>u_4</math>)</i> |
| $X_1 + X_2 \xrightarrow{0.10} \text{OUT}$              | <i>Rate: MAK(<math>k=0.1023</math>)</i>                |
| $X_1 + X_3 \xrightarrow{11.48} X_3$                    | <i>Rate: MAK(<math>k=11.4839</math>)</i>               |
| $X_2 + X_3 \xrightarrow{5.53} \text{OUT}$              | <i>Rate: MAK(<math>k=5.5349</math>)</i>                |
| $X_3 + X_4 \xrightarrow{0.21} \text{OUT}$              | <i>Rate: MAK(<math>k=0.2072</math>)</i>                |
| $X_4 + X_4 \xrightarrow{0.77} X_4$                     | <i>Rate: MAK(<math>k=0.7732</math>)</i>                |
| $\text{OUT} + \text{OUT} \xrightarrow{0.51} \emptyset$ | <i>Rate: MAK(<math>k=0.5060</math>)</i>                |

### 5.3 Configuration: 6 Species, 6 Reactions, non-zero initial condition

#### I/O CRN 1

**Inputs:**  $\{u_1, u_2, u_3, u_4\}$     **Species:**  $\{X_1, X_2, X_3, X_4, X_5\}$     **Output:**  $\text{OUT} = X_5$

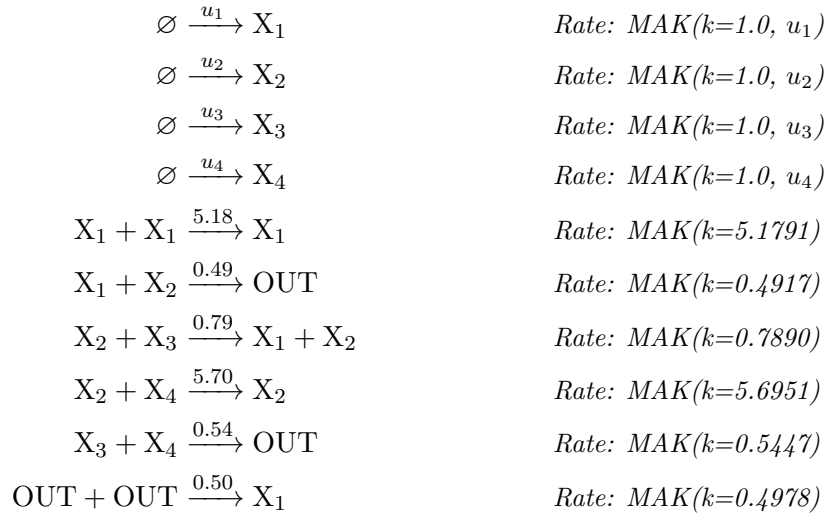

#### I/O CRN 3

**Inputs:**  $\{u_1, u_2, u_3, u_4\}$     **Species:**  $\{\text{OUT}, X_1, X_2, X_3, X_4\}$     **Output:**  $\text{OUT} = X_5$

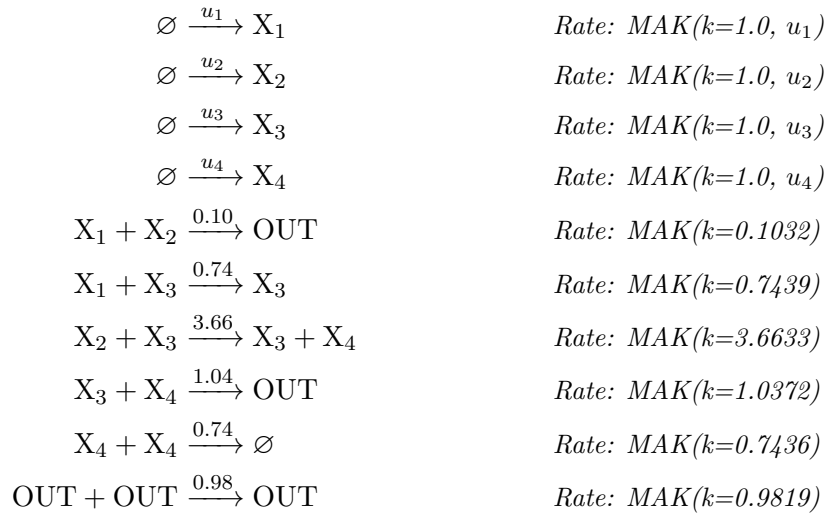

## I/O CRN 8

**Inputs:**  $\{u_1, u_2, u_3, u_4\}$     **Species:**  $\{X_1, X_2, X_3, X_4, X_5\}$     **Output:**  $OUT = X_5$

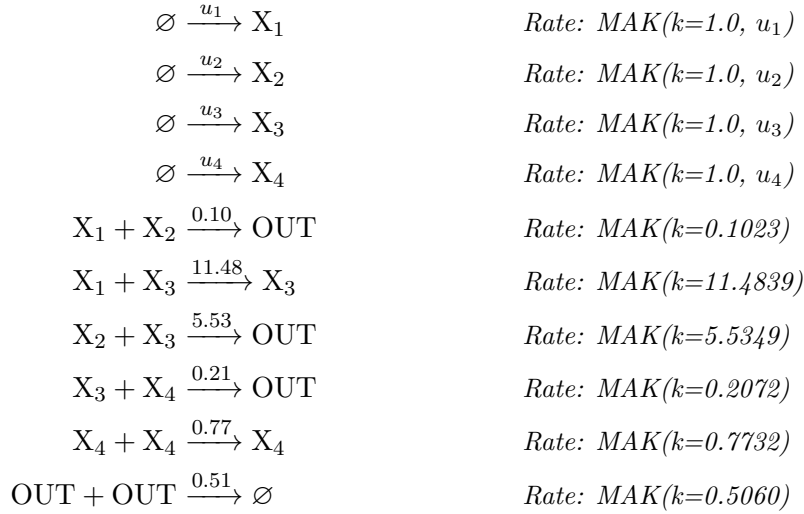

## 5.4 Configuration: 6 Species, 6 Reactions (Hill Functions)

### I/O CRN 1

**Loss:** 0.00114

**Inputs:**  $\{u_1, u_2, u_3, u_4\}$     **Species:**  $\{X_1, X_2, X_3, X_4, X_5, X_6\}$     **Output:**  $OUT = X_6$

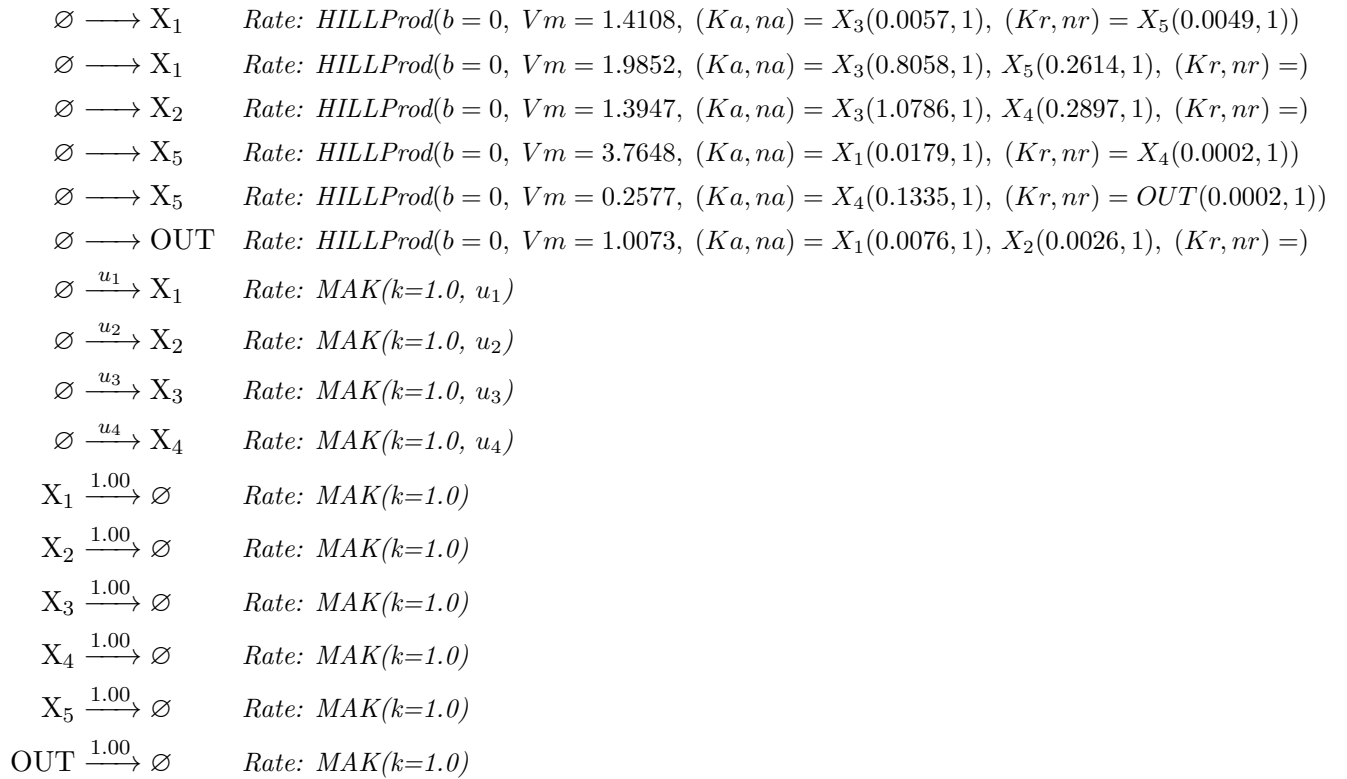

### I/O CRN 15

**Loss:** 0.00195

**Inputs:**  $\{u_1, u_2, u_3, u_4\}$     **Species:**  $\{X_1, X_2, X_3, X_4, X_5, X_6\}$     **Output:**  $OUT = X_6$

|                                    |                                                                                              |
|------------------------------------|----------------------------------------------------------------------------------------------|
| $\emptyset \longrightarrow X_1$    | Rate: $HILLProd(b = 0, Vm = 2.2641, (Ka, na) = X_3(0.0129, 1), X_5(0.0077, 1), (Kr, nr) = )$ |
| $\emptyset \longrightarrow X_2$    | Rate: $HILLProd(b = 0, Vm = 1.3628, (Ka, na) = X_3(0.0211, 1), X_4(0.5656, 1), (Kr, nr) = )$ |
| $\emptyset \longrightarrow X_5$    | Rate: $HILLProd(b = 0, Vm = 0.9270, (Ka, na) = , (Kr, nr) = X_4(0.0017, 1), X_5(0.0218, 1))$ |
| $\emptyset \longrightarrow X_5$    | Rate: $HILLProd(b = 0, Vm = 0.8529, (Ka, na) = X_5(0.1611, 1), (Kr, nr) = OUT(0.0642, 1))$   |
| $\emptyset \longrightarrow X_5$    | Rate: $HILLProd(b = 0, Vm = 1.6412, (Ka, na) = OUT(0.2783, 1), X_2(0.0216, 1), (Kr, nr) = )$ |
| $\emptyset \longrightarrow OUT$    | Rate: $HILLProd(b = 0, Vm = 1.0160, (Ka, na) = X_1(0.0110, 1), X_2(0.0104, 1), (Kr, nr) = )$ |
| $\emptyset \xrightarrow{u_1} X_1$  | Rate: $MAK(k=1.0, u_1)$                                                                      |
| $\emptyset \xrightarrow{u_2} X_2$  | Rate: $MAK(k=1.0, u_2)$                                                                      |
| $\emptyset \xrightarrow{u_3} X_3$  | Rate: $MAK(k=1.0, u_3)$                                                                      |
| $\emptyset \xrightarrow{u_4} X_4$  | Rate: $MAK(k=1.0, u_4)$                                                                      |
| $X_1 \xrightarrow{1.00} \emptyset$ | Rate: $MAK(k=1.0)$                                                                           |
| $X_2 \xrightarrow{1.00} \emptyset$ | Rate: $MAK(k=1.0)$                                                                           |
| $X_3 \xrightarrow{1.00} \emptyset$ | Rate: $MAK(k=1.0)$                                                                           |
| $X_4 \xrightarrow{1.00} \emptyset$ | Rate: $MAK(k=1.0)$                                                                           |
| $X_5 \xrightarrow{1.00} \emptyset$ | Rate: $MAK(k=1.0)$                                                                           |
| $OUT \xrightarrow{1.00} \emptyset$ | Rate: $MAK(k=1.0)$                                                                           |

---

### I/O CRN 30

**Loss:** 0.00256

**Inputs:**  $\{u_1, u_2, u_3, u_4\}$     **Species:**  $\{X_1, X_2, X_3, X_4, X_5, X_6\}$     **Output:**  $OUT = X_6$

|                                    |                                                                                              |
|------------------------------------|----------------------------------------------------------------------------------------------|
| $\emptyset \longrightarrow X_1$    | Rate: $HILLProd(b = 0, Vm = 1.1414, (Ka, na) = X_3(0.0044, 1), X_5(0.1256, 1), (Kr, nr) = )$ |
| $\emptyset \longrightarrow X_2$    | Rate: $HILLProd(b = 0, Vm = 4.2466, (Ka, na) = X_3(0.0607, 1), X_4(0.0016, 1), (Kr, nr) = )$ |
| $\emptyset \longrightarrow X_5$    | Rate: $HILLProd(b = 0, Vm = 0.3768, (Ka, na) = X_4(0.0061, 1), (Kr, nr) = X_5(0.0001, 1))$   |
| $\emptyset \longrightarrow X_5$    | Rate: $HILLProd(b = 0, Vm = 0.8472, (Ka, na) = OUT(0.0333, 1), (Kr, nr) = X_5(0.1009, 1))$   |
| $\emptyset \longrightarrow X_5$    | Rate: $HILLProd(b = 0, Vm = 0.7262, (Ka, na) = X_4(0.0015, 1), X_5(0.0005, 1), (Kr, nr) = )$ |
| $\emptyset \longrightarrow OUT$    | Rate: $HILLProd(b = 0, Vm = 1.0044, (Ka, na) = X_1(0.0007, 1), X_2(0.0089, 1), (Kr, nr) = )$ |
| $\emptyset \xrightarrow{u_1} X_1$  | Rate: $MAK(k=1.0, u_1)$                                                                      |
| $\emptyset \xrightarrow{u_2} X_2$  | Rate: $MAK(k=1.0, u_2)$                                                                      |
| $\emptyset \xrightarrow{u_3} X_3$  | Rate: $MAK(k=1.0, u_3)$                                                                      |
| $\emptyset \xrightarrow{u_4} X_4$  | Rate: $MAK(k=1.0, u_4)$                                                                      |
| $X_1 \xrightarrow{1.00} \emptyset$ | Rate: $MAK(k=1.0)$                                                                           |
| $X_2 \xrightarrow{1.00} \emptyset$ | Rate: $MAK(k=1.0)$                                                                           |
| $X_3 \xrightarrow{1.00} \emptyset$ | Rate: $MAK(k=1.0)$                                                                           |
| $X_4 \xrightarrow{1.00} \emptyset$ | Rate: $MAK(k=1.0)$                                                                           |
| $X_5 \xrightarrow{1.00} \emptyset$ | Rate: $MAK(k=1.0)$                                                                           |
| $OUT \xrightarrow{1.00} \emptyset$ | Rate: $MAK(k=1.0)$                                                                           |

## 6 Task: Oscillators

This section details the In-Silico Optimized Chemical Reaction Networks (I/O CRNs) discovered for the Oscillator task, where the system is designed to produce sustained periodic fluctuations in the output species.

### 6.1 Configuration: 3 Species, 6 Reactions

#### I/O CRN 8

Loss: 0.00587

Inputs:  $\{u_1\}$     Species:  $\{X_1, X_2, X_3\}$     Output:  $X_3$

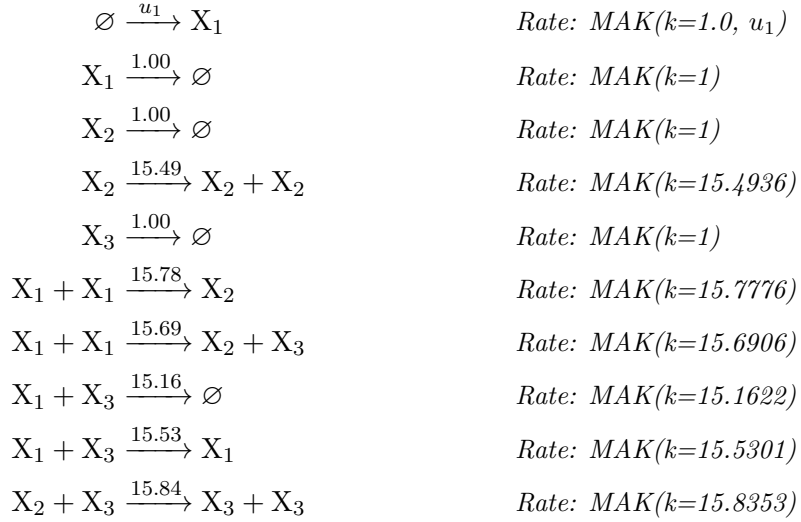

#### I/O CRN 10

Loss: 0.00617

Inputs:  $\{u_1\}$     Species:  $\{X_1, X_2, X_3\}$     Output:  $X_3$

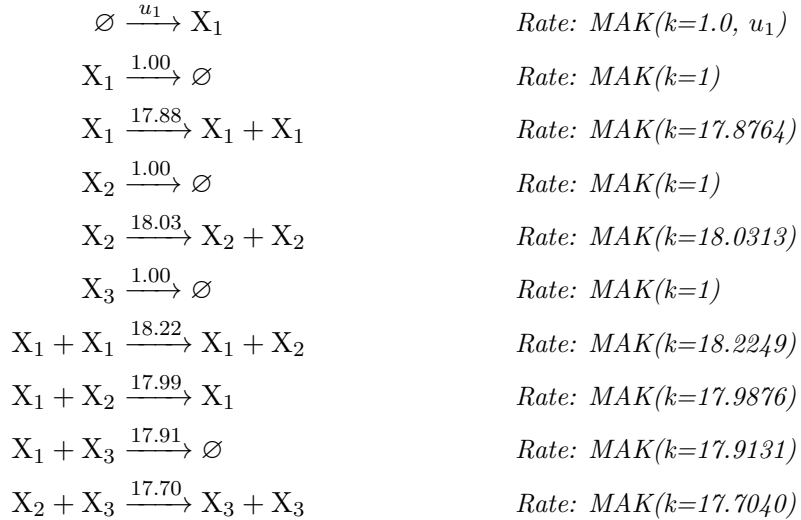

## I/O CRN 100

Loss: 0.01307

Inputs:  $\{u_1\}$     Species:  $\{X_1, X_2, X_3\}$     Output:  $X_3$

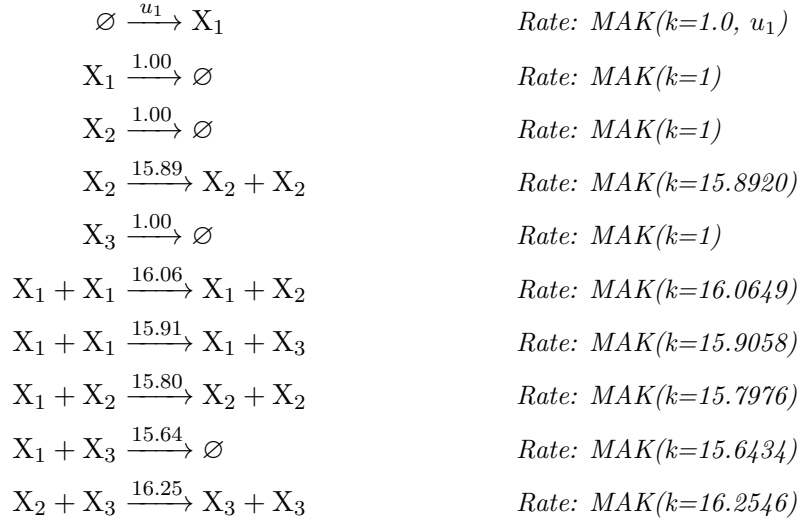

## 6.2 Configuration: 3 Species, 6 Reactions (Frequency Tuning)

### I/O CRN 3

Loss: 0.06399

Inputs:  $\{u_1\}$     Species:  $\{X_1, X_2, X_3\}$     Output:  $X_3$

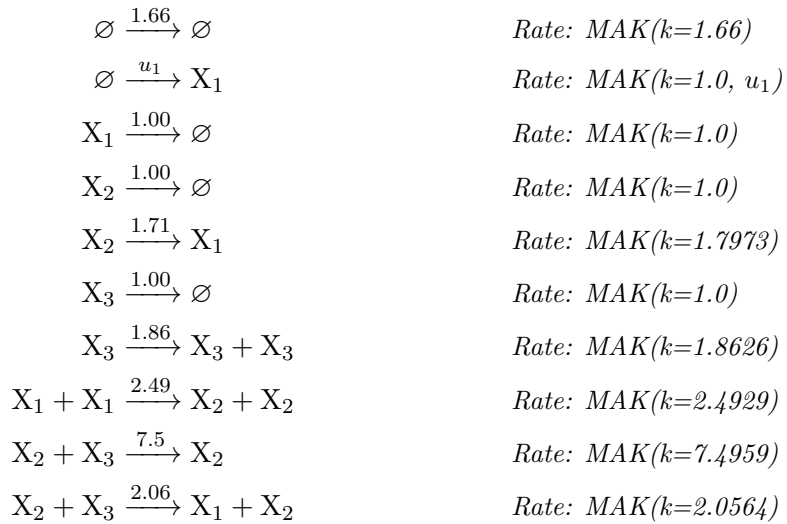

---

### I/O CRN 39

Loss: 0.07286

Inputs:  $\{u_1\}$     Species:  $\{X_1, X_2, X_3\}$     Output:  $X_3$

|                                          |                                           |
|------------------------------------------|-------------------------------------------|
| $\emptyset \xrightarrow{u_1} X_1$        | <i>Rate: MAK(k=1.0, <math>u_1</math>)</i> |
| $X_1 \xrightarrow{1.00} \emptyset$       | <i>Rate: MAK(k=1.0)</i>                   |
| $X_2 \xrightarrow{1.00} \emptyset$       | <i>Rate: MAK(k=1.0)</i>                   |
| $X_3 \xrightarrow{1.00} \emptyset$       | <i>Rate: MAK(k=1.0)</i>                   |
| $X_3 \xrightarrow{2.13} X_1 + X_3$       | <i>Rate: MAK(k=2.1282)</i>                |
| $X_1 + X_1 \xrightarrow{4.81} X_1 + X_3$ | <i>Rate: MAK(k=4.8111)</i>                |
| $X_1 + X_1 \xrightarrow{2.62} X_3 + X_3$ | <i>Rate: MAK(k=2.6216)</i>                |
| $X_1 + X_3 \xrightarrow{2.58} X_1 + X_1$ | <i>Rate: MAK(k=2.5795)</i>                |
| $X_2 + X_3 \xrightarrow{4.8} X_2 + X_2$  | <i>Rate: MAK(k=4.7978)</i>                |

---

## I/O CRN 51

Loss: 0.07583

Inputs:  $\{u_1\}$     Species:  $\{X_1, X_2, X_3\}$     Output:  $X_3$

|                                          |                                           |
|------------------------------------------|-------------------------------------------|
| $\emptyset \xrightarrow{u_1} X_1$        | <i>Rate: MAK(k=1.0, <math>u_1</math>)</i> |
| $X_1 \xrightarrow{1.00} \emptyset$       | <i>Rate: MAK(k=1.0)</i>                   |
| $X_2 \xrightarrow{1.00} \emptyset$       | <i>Rate: MAK(k=1.0)</i>                   |
| $X_3 \xrightarrow{1.00} \emptyset$       | <i>Rate: MAK(k=1.0)</i>                   |
| $X_3 \xrightarrow{2.81} X_1 + X_3$       | <i>Rate: MAK(k=2.8096)</i>                |
| $X_1 + X_1 \xrightarrow{3.10} X_3 + X_3$ | <i>Rate: MAK(k=3.0999)</i>                |
| $X_1 + X_2 \xrightarrow{3.66} X_2$       | <i>Rate: MAK(k=3.6616)</i>                |
| $X_1 + X_3 \xrightarrow{2.21} X_1 + X_1$ | <i>Rate: MAK(k=2.2070)</i>                |
| $X_2 + X_3 \xrightarrow{6.77} X_2 + X_2$ | <i>Rate: MAK(k=6.7750)</i>                |
| $X_3 + X_3 \xrightarrow{1.68} X_1 + X_3$ | <i>Rate: MAK(k=1.6773)</i>                |

## 7 Task: Habituation and Sensitization

This section reports the In-Silico Optimized Chemical Reaction Networks (I/O CRNs) discovered for habituation and sensitization. In both tasks, the system is stimulated by repeated pulses of the input  $u_1$  (with an inter-train OFF gap), and the output species  $X_3$  is optimized to exhibit either decreasing (habituation) or increasing (sensitization) peak responses across successive pulses.

## 7.1 Habituation

### I/O CRN 1

**Inputs:**  $\{u_1\}$     **Species:**  $\{X_1, X_2, X_3\}$     **Output:**  $X_3$

|                                          |                                           |
|------------------------------------------|-------------------------------------------|
| $\emptyset \xrightarrow{1.23} \emptyset$ | <i>Rate: MAK(<math>k=1.2254</math>)</i>   |
| $\emptyset \xrightarrow{u_1} X_1$        | <i>Rate: MAK(<math>k=1.0, u_1</math>)</i> |
| $\emptyset \xrightarrow{0.10} X_2$       | <i>Rate: MAK(<math>k=0.1</math>)</i>      |
| $X_1 \xrightarrow{0.10} \emptyset$       | <i>Rate: MAK(<math>k=0.1</math>)</i>      |
| $X_1 \xrightarrow{51.83} X_1 + X_3$      | <i>Rate: MAK(<math>k=51.8283</math>)</i>  |
| $X_2 \xrightarrow{0.10} \emptyset$       | <i>Rate: MAK(<math>k=0.1</math>)</i>      |
| $X_3 \xrightarrow{0.10} \emptyset$       | <i>Rate: MAK(<math>k=0.1</math>)</i>      |
| $X_1 + X_3 \xrightarrow{0.73} X_3$       | <i>Rate: MAK(<math>k=0.7332</math>)</i>   |
| $X_2 + X_3 \xrightarrow{0.76} X_2 + X_2$ | <i>Rate: MAK(<math>k=0.7588</math>)</i>   |
| $X_3 + X_3 \xrightarrow{5.88} \emptyset$ | <i>Rate: MAK(<math>k=5.8811</math>)</i>   |

---

### I/O CRN 5

**Inputs:**  $\{u_1\}$     **Species:**  $\{X_1, X_2, X_3\}$     **Output:**  $X_3$

|                                          |                                           |
|------------------------------------------|-------------------------------------------|
| $\emptyset \xrightarrow{2.44} \emptyset$ | <i>Rate: MAK(<math>k=2.4425</math>)</i>   |
| $\emptyset \xrightarrow{u_1} X_1$        | <i>Rate: MAK(<math>k=1.0, u_1</math>)</i> |
| $\emptyset \xrightarrow{0.10} X_2$       | <i>Rate: MAK(<math>k=0.1</math>)</i>      |
| $X_1 \xrightarrow{0.10} \emptyset$       | <i>Rate: MAK(<math>k=0.1</math>)</i>      |
| $X_1 \xrightarrow{12.26} X_1 + X_3$      | <i>Rate: MAK(<math>k=12.2619</math>)</i>  |
| $X_2 \xrightarrow{0.10} \emptyset$       | <i>Rate: MAK(<math>k=0.1</math>)</i>      |
| $X_3 \xrightarrow{0.10} \emptyset$       | <i>Rate: MAK(<math>k=0.1</math>)</i>      |
| $X_1 + X_3 \xrightarrow{0.54} X_3$       | <i>Rate: MAK(<math>k=0.5446</math>)</i>   |
| $X_1 + X_3 \xrightarrow{0.28} X_2 + X_3$ | <i>Rate: MAK(<math>k=0.2842</math>)</i>   |
| $X_2 + X_3 \xrightarrow{0.46} X_2 + X_2$ | <i>Rate: MAK(<math>k=0.4598</math>)</i>   |

---

## I/O CRN 7

**Inputs:**  $\{u_1\}$     **Species:**  $\{X_1, X_2, X_3\}$     **Output:**  $X_3$

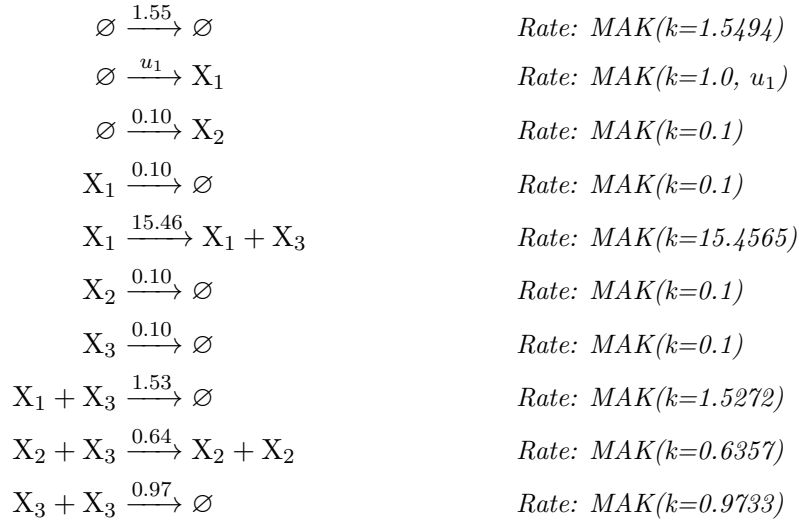

## 7.2 Sensitization

### I/O CRN 1

**Inputs:**  $\{u_1\}$     **Species:**  $\{X_1, X_2, X_3\}$     **Output:**  $X_3$

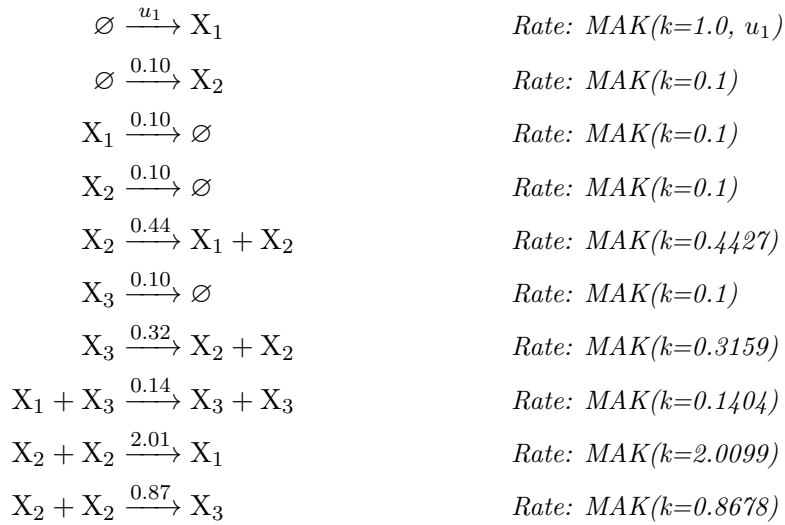

#### I/O CRN 4

**Inputs:**  $\{u_1\}$     **Species:**  $\{X_1, X_2, X_3\}$     **Output:**  $X_3$

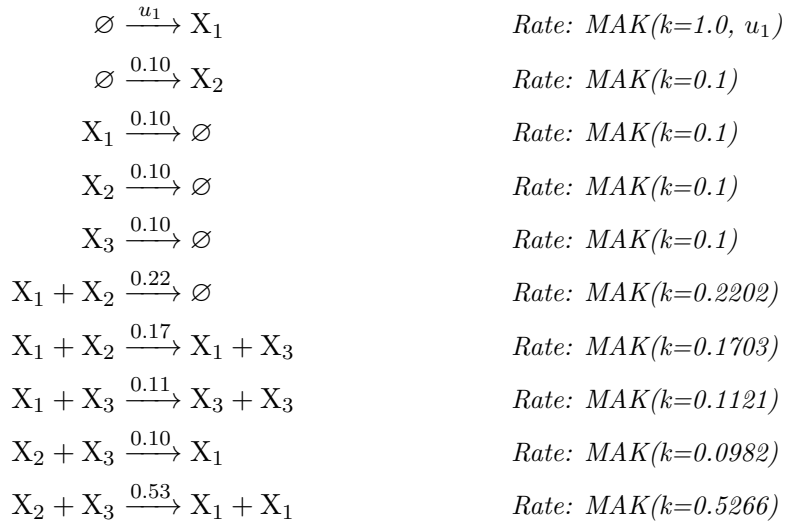

#### I/O CRN 7

**Inputs:**  $\{u_1\}$     **Species:**  $\{X_1, X_2, X_3\}$     **Output:**  $X_3$

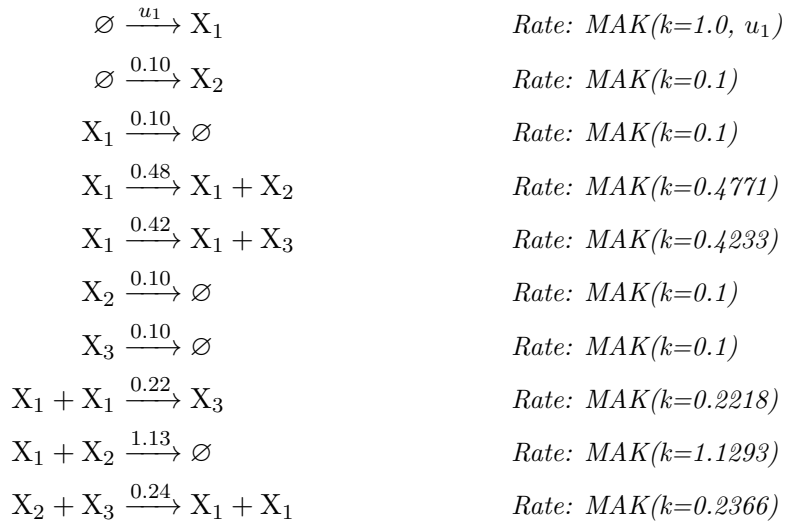

Supplement: Supplementary file 1 [file Supplementary_Material.pdf]
